# Supplementary material for: Decomposed Mean-Field Simulations of Local Properties in Condensed Phases
Source: arXiv:2104.12480 ancillary file (2021-06-28)
Supplement: Supplementary file 1 [file si.pdf]

# Supporting Information: Decomposed Mean-Field Simulations of Local Properties in Condensed Phases

Janus J. Eriksen*

*DTU Chemistry, Technical University of Denmark*

*Kemitorvet Bldg. 206, DK–2800, Kgs. Lyngby, Denmark*

E-mail: janus@kemi.dtu.dk

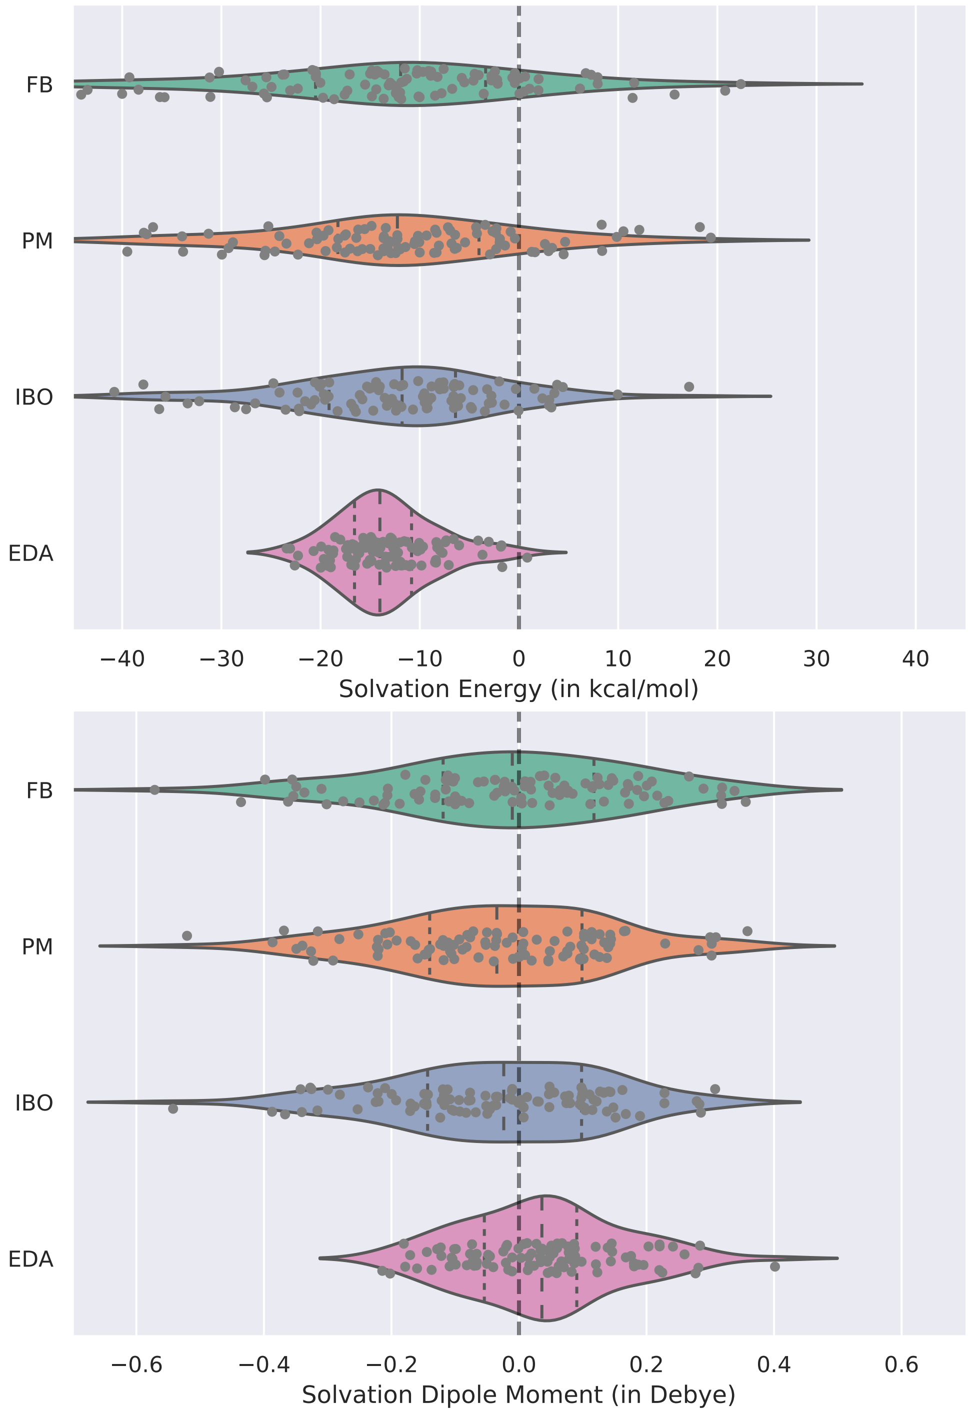


**Figure S1:** Violin distributions of the energies and dipole moments of $H_2O$ in the TIP3P/flex sampling ($r = 4.0$ Å), as calculated at the B3LYP/pc-1 level of theory, TIP3P background point charges, and on the basis of various spatially localized MOs (FB,[S1] PM,[S2] and IBOs[S3]) as well as Nakai's energy density analysis (EDA) partitioning.[S4,S5] Partial charges (atomic weights) are derived in an IAO basis in all cases but the latter (EDA), which relies only on a predefined partitioning of the AOs.

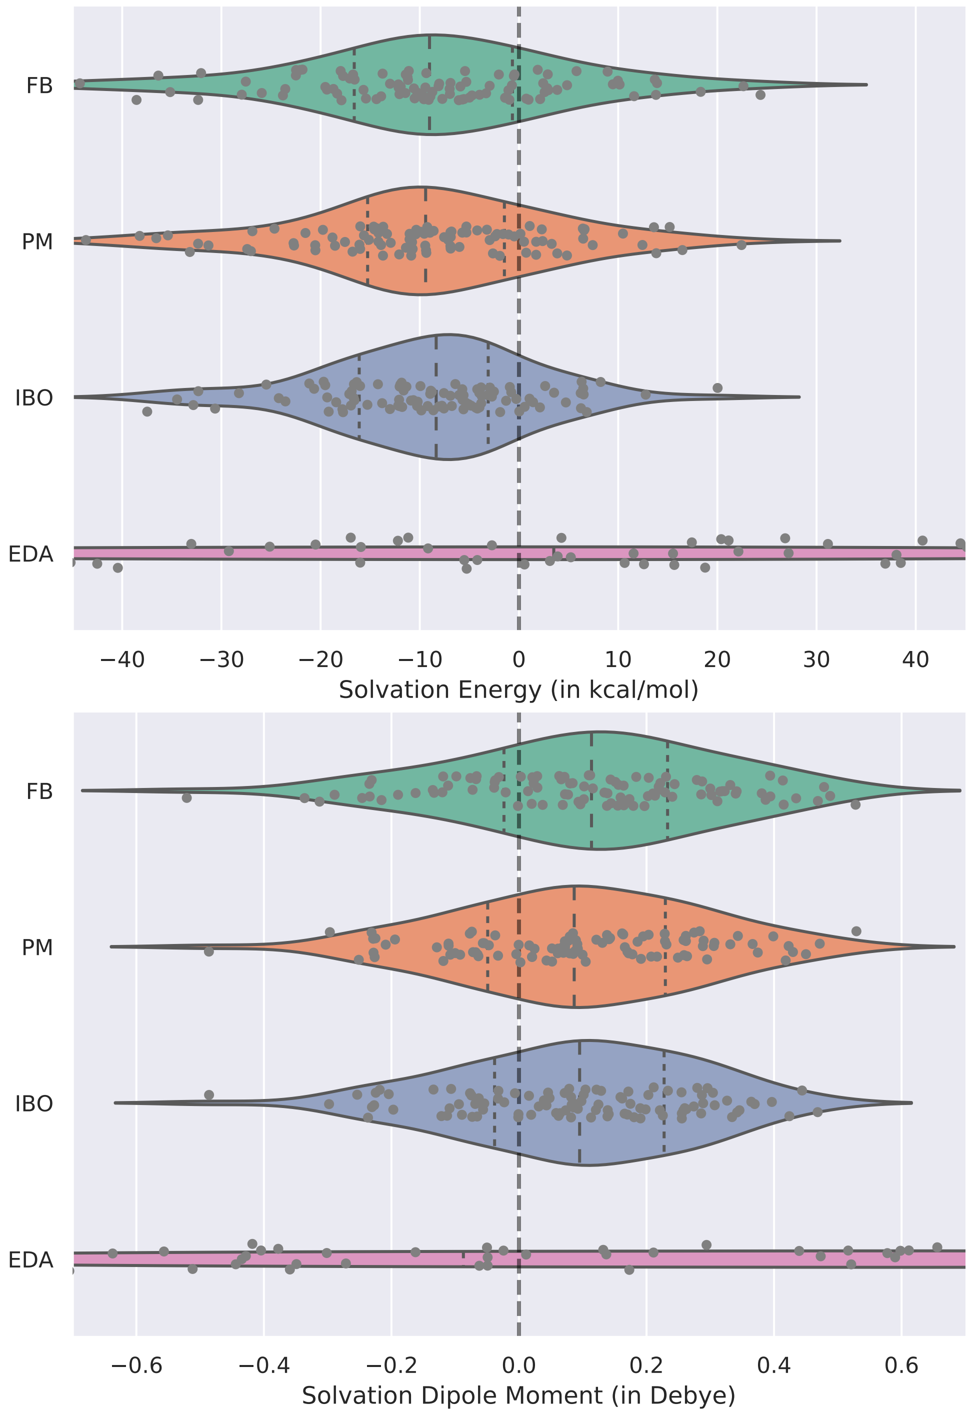


**Figure S2:** Same as in Fig. S1, but calculated at the B3LYP/aug-pc-1 level of theory.

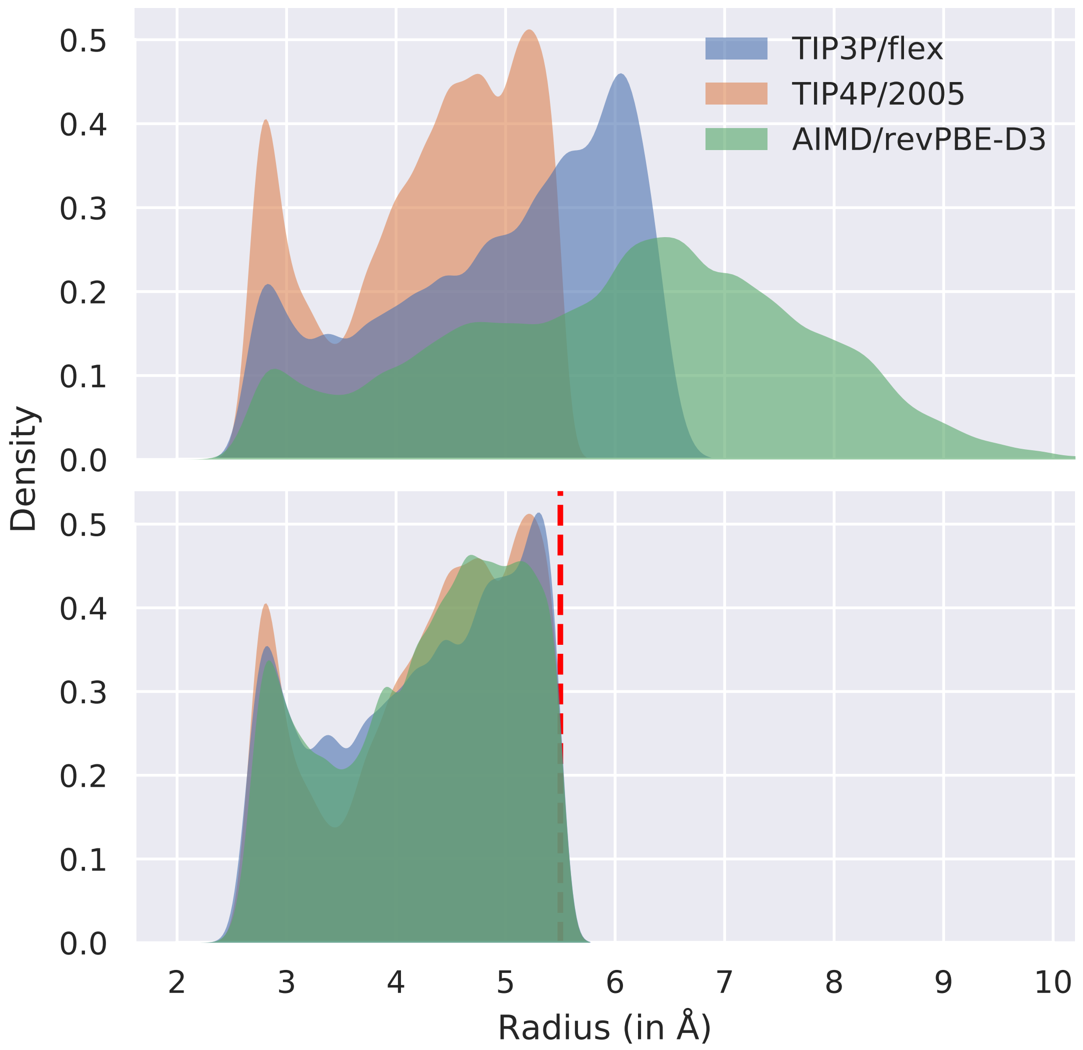


**Figure S3:** Distributions of neighbouring monomers, as represented by kernel density estimations (KDEs) and measured as O–O distances outwards from a central monomer unit in the three samplings. In the lower panel, the distributions have been restricted to a threshold radius of $R = 5.5$ Å.

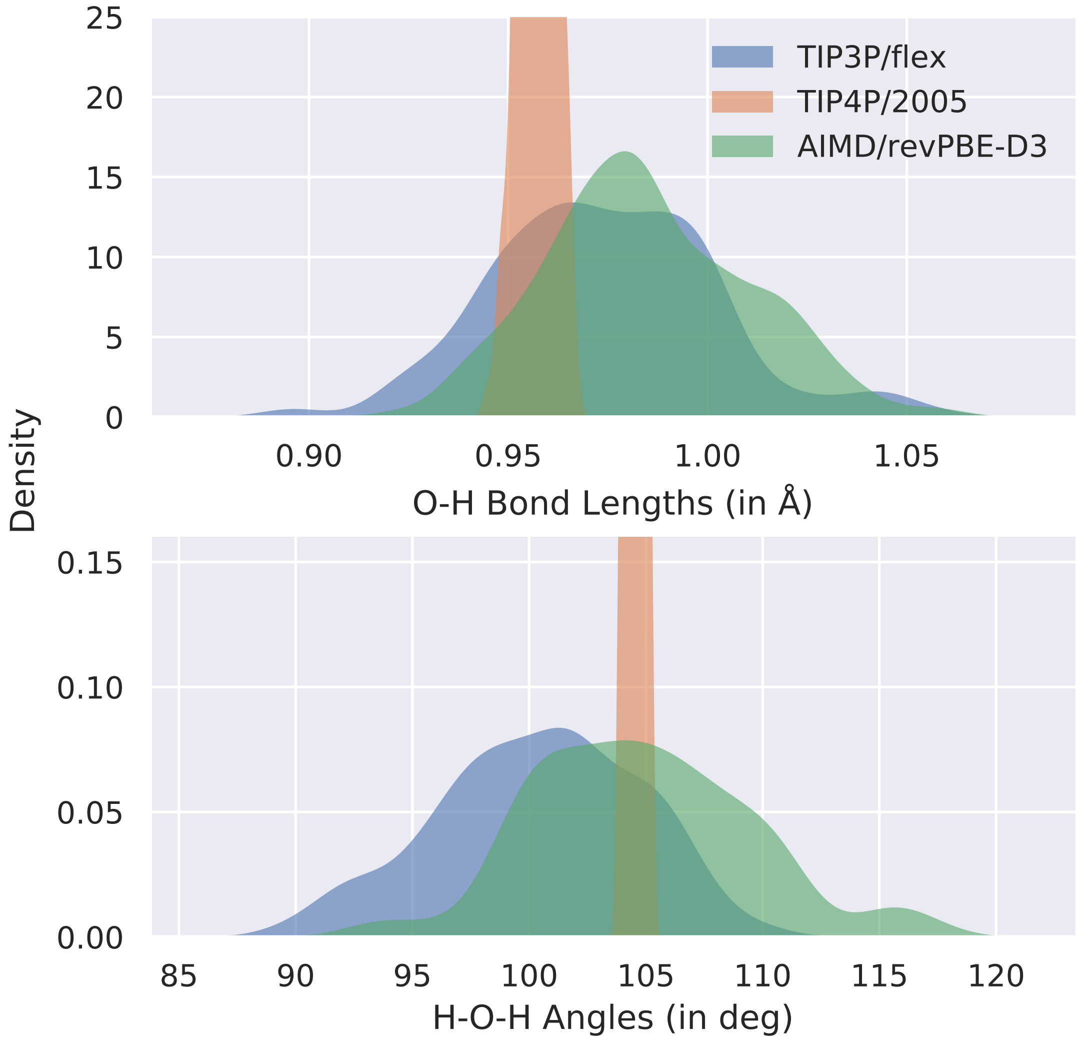


**Figure S4:** Distributions of O–H bond lengths and ∠(H–O–H) angles for the chosen central monomer units in the three different samplings, as represented by KDEs.

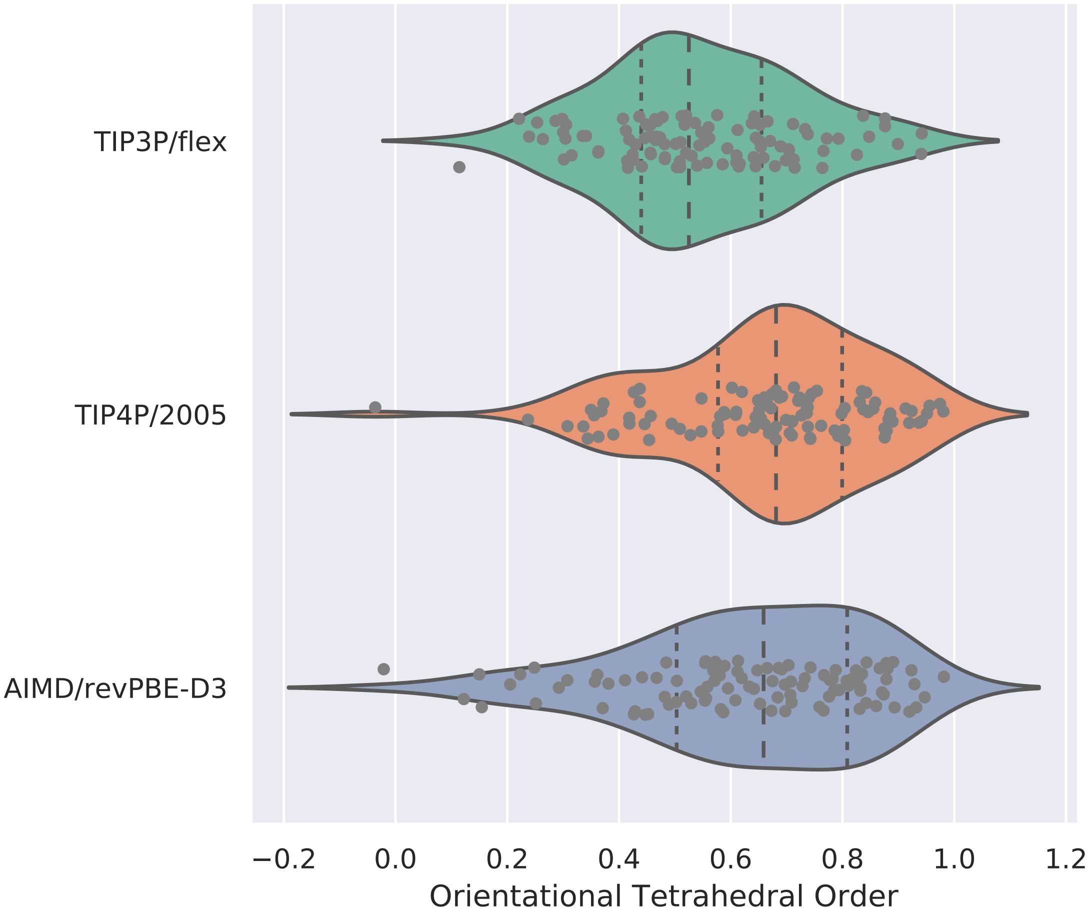


**Figure S5:** Violin plots (with quartiles of the underlying distribution displayed) of the orientational tetrahedral order[S6,S7] (OTO) within each of the three bulk samplings, as calculated by the expression, $q = 1 - \frac{3}{8}\sum_{j=1}^{3}\sum_{k=j+1}^{4}(\cos\psi_{jk} + \frac{1}{3})^2$. Here, $\psi_{jk}$ is the angle formed by the lines joining the oxygen atom of the central water molecule under consideration and its neighbour oxygen atoms $j$ and $k$ (of which a total of 4 are considered). The average value of $q$ varies from 0 for an ideal gas to 1 in the case of a regular tetrahedron.

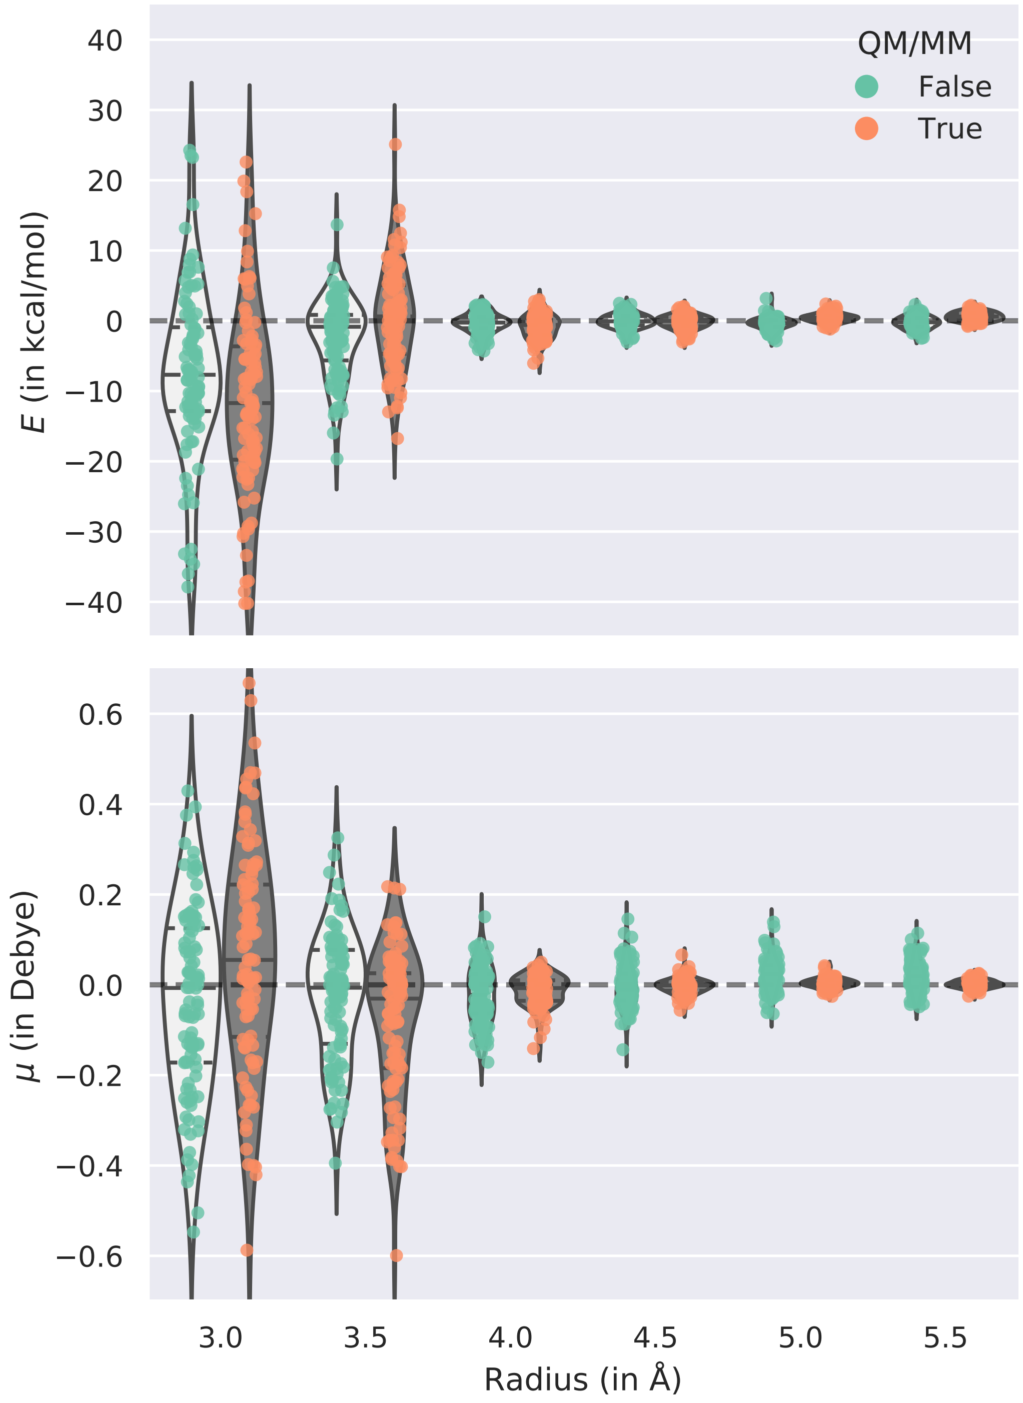


**Figure S6:** Convergence of solvation energies and dipole moments of $H_2O$ in the TIP3P/flex sampling, as calculated by coarse-grained samplings at the B3LYP/pc-1 level of theory. A combination of IAOs and IBOs is used at all radii. Results are presented in terms of the change to the properties upon moving outwards from a central bulk monomer unit in vacuum, and results are presented for samplings in the absence/presence of background point charges.

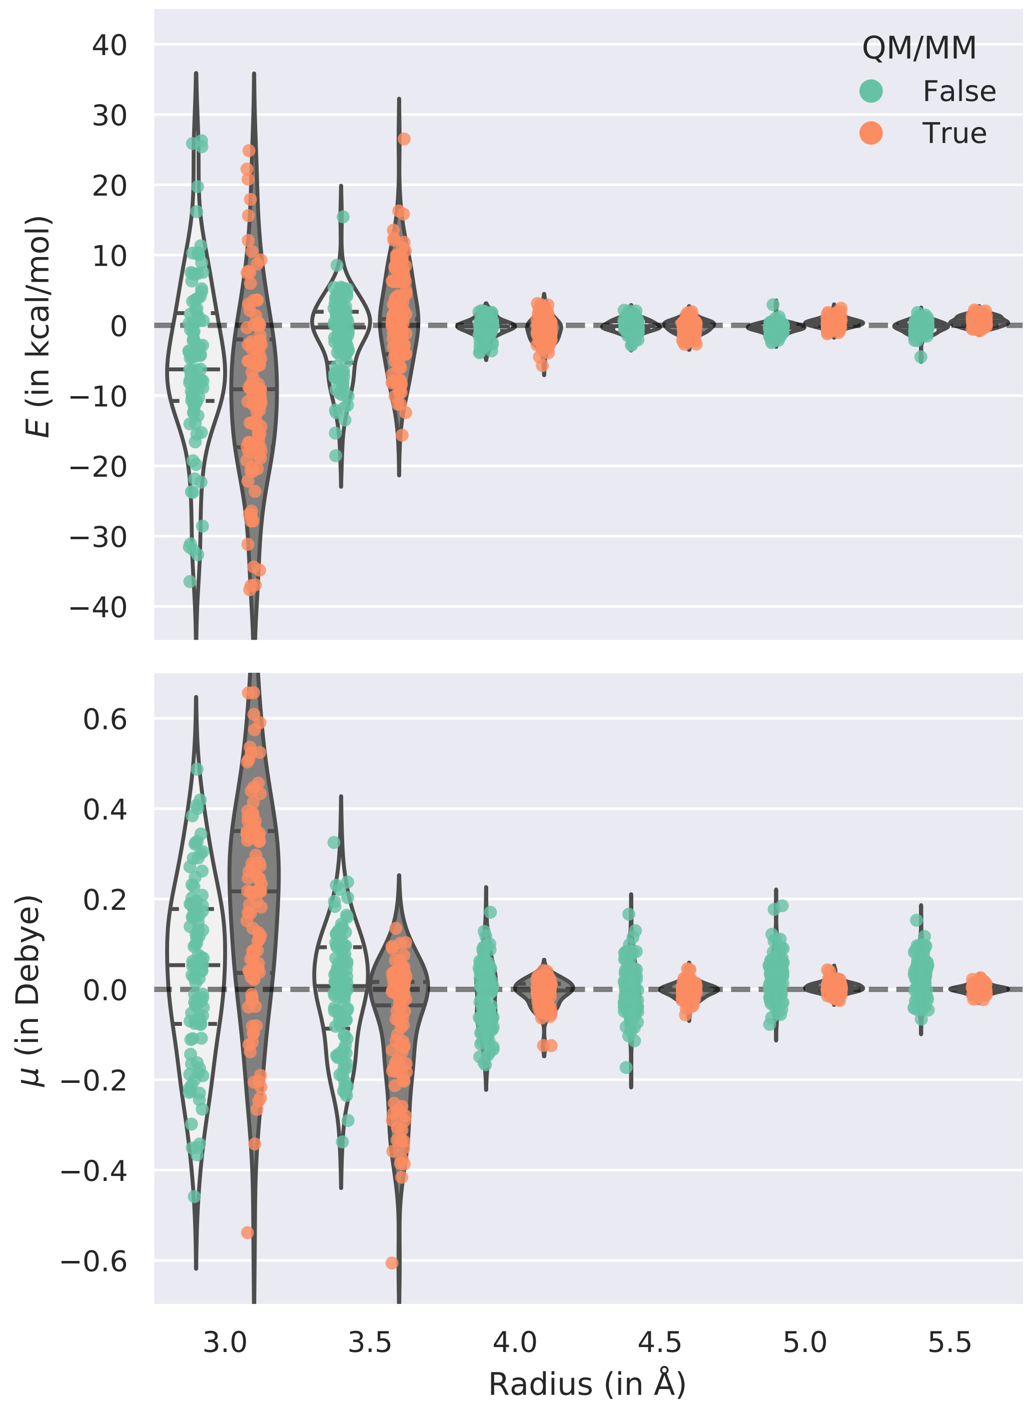


**Figure S7:** Same as in Fig. S6, but computed at the B3LYP/aug-pc-1 level of theory.

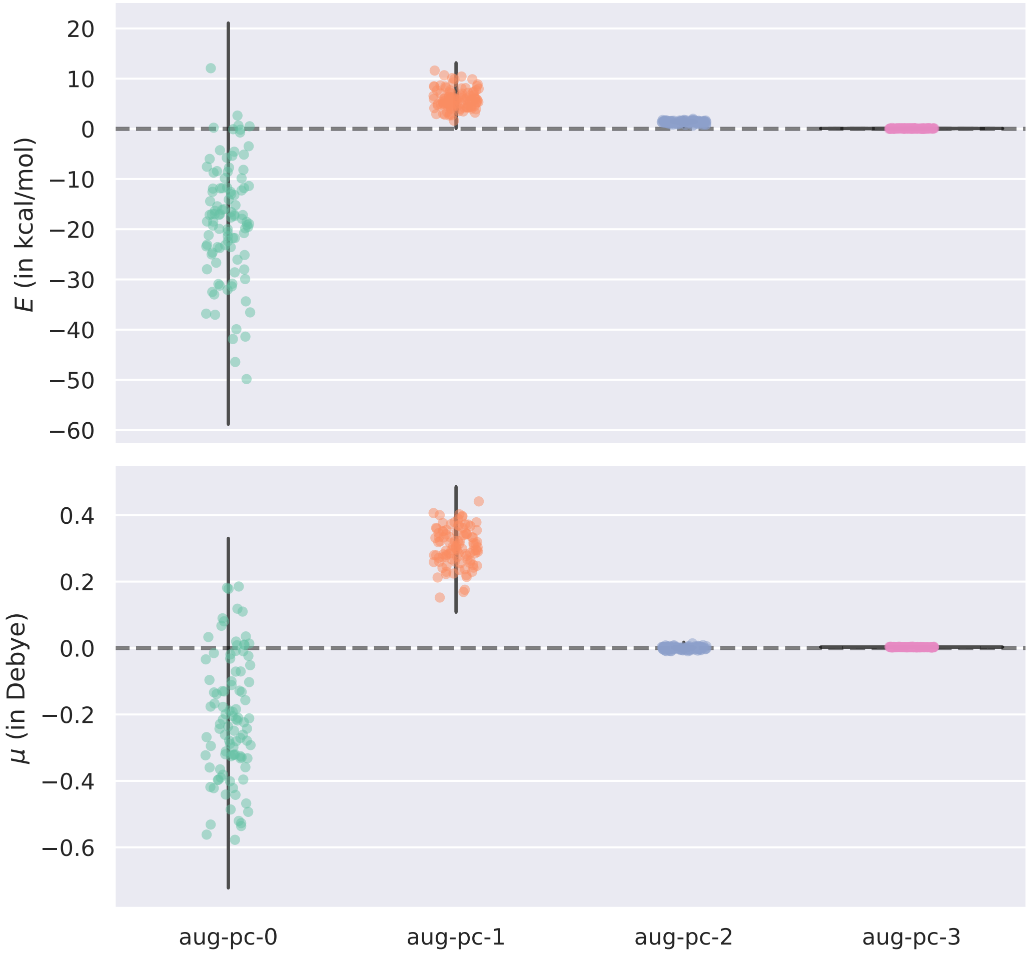


**Figure S8:** Convergence of solvation energies and dipole moments of $H_2O$ in the AIMD/revPBE-D3 sampling, as calculated at the B3LYP/aug-pc-$x$ level of theory ($x = 0$–3) and measured against results in the largest aug-pc-3 basis set.

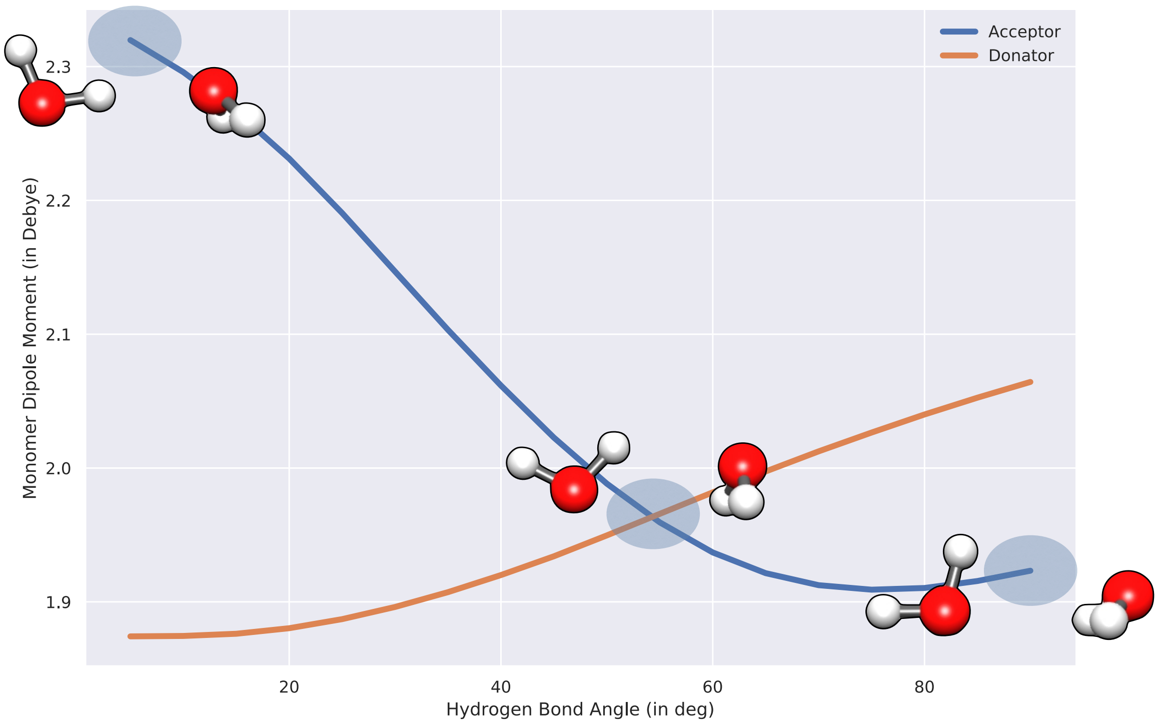


**Figure S9:** Decomposed molecular dipole moments along an optimized potential energy scan of the water dimer ($C_s$ symmetry), calculated at the B3LYP/aug-pc-1 level of theory. The acceptor is situated furthest to the right in all insets, and *vice versa* for the donator.

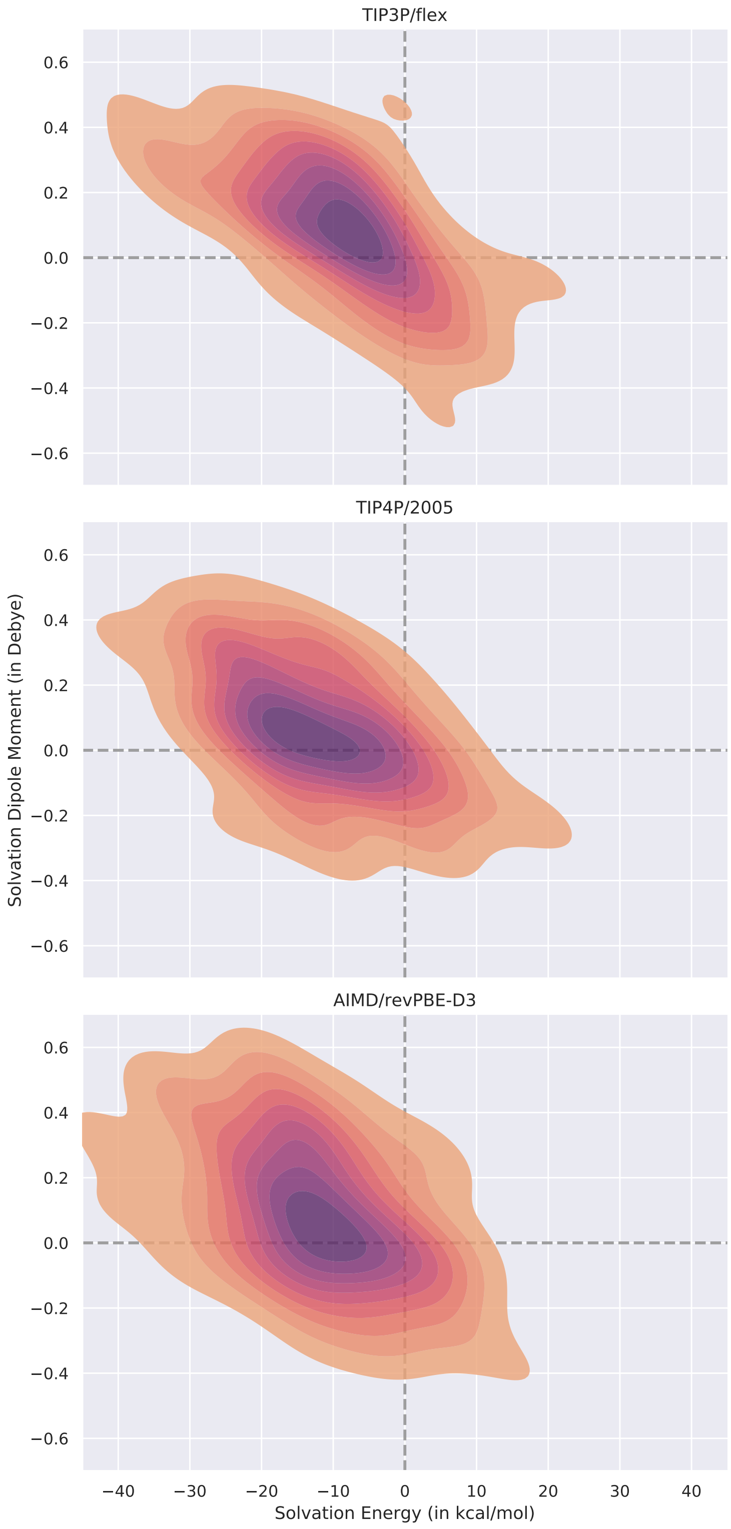


**Figure S10:** Distributions of solvation energies and dipole moments of $H_2O$ in all three samplings at $r = 4.0$ Å, as calculated at the B3LYP/aug-pc-1 level of theory.

# References

(S1) Foster, J. M.; Boys, S. F. Canonical Configurational Interaction Procedure. Rev. Mod. Phys. **1960**, 32, 300.

(S2) Pipek, J.; Mezey, P. G. A Fast Intrinsic Localization Procedure Applicable for *Ab Initio* and Semiempirical Linear Combination of Atomic Orbital Wave Functions. J. Chem. Phys. **1989**, 90, 4916.

(S3) Knizia, G. Intrinsic Atomic Orbitals: An Unbiased Bridge Between Quantum Theory and Chemical Concepts. J. Chem. Theory Comput. **2013**, 9, 4834.

(S4) Nakai, H. Energy Density Analysis with Kohn-Sham Orbitals. Chem. Phys. Lett. **2002**, 363, 73.

(S5) Kikuchi, Y.; Imamura, Y.; Nakai, H. One-Body Energy Decomposition Schemes Revisited: Assessment of Mulliken-, Grid-, and Conventional Energy Density Analyses. Int. J. Quantum Chem. **2009**, 109, 2464.

(S6) Chau, P.-L.; Hardwick, A. J. A New Order Parameter for Tetrahedral Configurations. Mol. Phys. **1998**, 93, 511.

(S7) Errington, J. R.; Debenedetti, P. G. Relationship Between Structural Order and the Anomalies of Liquid Water. Nature **2001**, 409, 318.
